# Supplementary material for: Refinement Reflection: Complete Verification with SMT
Source: arXiv:1711.03842 source file (2017-11-09)
Supplement: Supplementary file 1 [file Formalism.Appendix.tex]

\section{Formalism}

\begin{figure}[t!]
\centering
$$
\begin{array}{rrcl}
\emphbf{Values} \quad 
  & w & ::=&  c 
             \spmid \efun{x}{\typ}{e} \spmid D\ \overline{e}
\\[0.03in] 

\emphbf{Expressions} \quad 
  & e & ::=     & w \spmid x 
                  \spmid \eapp{e}{e}      \\
  & & \spmid & \ecase{x}{e}{\dc}{\overline{x}}{e}
\\[0.03in]

\emphbf{Program} \quad 
  & \prog & ::= & e \spmid \elet{x}{e}{\gtyp}{[L]}{\prog}\\
  & & \spmid & \eletrec{x}{e}{\gtyp}{[L]}{\prog}
\\[0.03in] 

\emphbf{Logical Labels} \quad 
  & L & ::= & A \spmid M \spmid I
\\[0.03in] 

\emphbf{Refinements} \quad
  & r 
  & ::= & e
\\[0.03in] 
  
\emphbf{Operators} \quad
  & \odot 
  & ::= & = \spmid  \not = \spmid \leq \spmid < \spmid \geq \spmid >
\\[0.03in] 

\emphbf{Constants} \quad
  & c 
  & ::= 
  & \land \spmid \lnot \spmid \odot  \\
  && \spmid &  0 \spmid 1 \spmid -1 \spmid \dots \\
  && \spmid & \etrue \spmid \efalse
\\[0.03in] 
  
\emphbf{Basic Types} \quad
  & \btyp
  & ::= 
  & \tint \spmid \tbool \spmid T 
\\[0.03in] 
  
\emphbf{Environment} \quad 
  & \env
  & ::= & \tbind{x}{\gtyp}, \env \spmid \emptyset
\\[0.03in]
 
\emphbf{Substitution} \quad 
  & \sub
  & ::= & \tbind{x}{\prog}, \sub \spmid \emptyset
\\[0.03in]

\emphbf{Refined Types} \quad 
  & \typ
  & ::=      & \tref{v}{\btyp}{\reft} \spmid \tfun{x}{\typ}{\typ}
\\[0.05in]
 
\emphbf{Context} \quad
  & C 
  & ::=
  & \bullet \spmid C\ e \spmid c\ C \spmid D\ \overline{e}\ C\ \overline{e}\\
  && \spmid & \ecase{y}{C}{\dc_i}{\overline{x}}{e_i}
\\[0.03in]

\end{array}
$$

\emphbf{Reductions}\hfill{\mbox{$\goesto{\prog}{\prog'}$}}
$$
\begin{array}{rcl}
C[\prog] &\hookrightarrow& C[\prog'],\quad \text{if}\ \goesto{\prog}{\prog'}\\
{c\ v}&\hookrightarrow&{\delta(c, v)}\\
{({\efun{x}{\typ}{e})}\ {e_x}}&\hookrightarrow&{e\subst{x}{e_x}}\\
{\ecase{y}{\dc_j\ \overline{e}}{\dc_i}{\overline{x_i}}{e_i}}&\hookrightarrow&
       {e_j\subst{y}{\dc_j\ \overline{e}}\subst{\overline{x_i}}{\overline{e}}}\\
{\elet{x}{e_x}{\gtyp}{[L]}{\prog}}&\hookrightarrow&{\prog\subst{x}{e}}\\
{\eletrec{x}{e_x}{\gtyp}{[L]}{\prog}}&\hookrightarrow&{\prog\subst{x}{\efix{x}\ {e_x}}}\\
{\efix{x}}&\hookrightarrow&{x\ (\efix{x})}
\end{array}
$$

\caption{\textbf{Syntax and Semantics of \corelan}}
\label{fig:syntax}
\end{figure}

\subsubsection{Axioms}
\begin{align*}
\embed{\eletrecopt{x}{e}{\gtyp}{A}{\prog}}
  &= \eletrecopt{x}{e}{\exacttype{\gtyp}{e}}{}{\embed{\prog}}\\
\embed{\eletrecopt{x}{e}{\gtyp}{\star}{\prog}}
  &= \eletrecopt{x}{e}{\gtyp}{\star}{\embed{\prog}}\\
\embed{e} &= e 
\end{align*}

\begin{align*}
\exacttype{\tref{v}{\btyp}{r}}{e} &= \tref{v}{\btyp}{r \land v = e}\\
\exacttype{\tfun{x}{\typ_x}{\typ}}{\efun{y}{}{e}} &=\tfun{x}{\typ_x}{\exacttype{\typ}{e\subst{y}{x}}} 
\end{align*}
